# Supplementary material for: libcll: an Extendable Python Toolkit for Complementary-Label Learning
Source: arXiv:2411.12276 source file (2024-11-19)
Supplement: Supplementary file 1 [file Appendix.tex]

\section*{Appendix}

\section{libcll Strategies}
\label{sec:strategies}
\begin{table}[ht]
\centering
\caption{Overview of strategies included in the \texttt{libcll} toolkit.}
% \vskip 0.15in
\label{tab:strategies}
\setlength{\tabcolsep}{10pt} % Default value: 6pt
 % Default value: 1
\resizebox{1\linewidth}{!}{%
\scalebox{0.50}{
\begin{tabular}{l|c|l}
\hline
Strategy & Type & Description \\
\hline
\multirow{2}{4em}{SCL~\cite{scl2020}} & NL & Surrogate Complementary Loss with negative log loss. \\
& EXP & Surrogate Complementary Loss with exponential loss. \\
\hline
\multirow{4}{4em}{URE~\cite{ishida2019complementarylabel}} & NN & Unbiased risk estimator with uniform transition matrix. \\
& GA & Gradient Ascent applied to the unbiased risk estimator with uniform transition matrix. \\
& TNN & Unbiased risk estimator with true transition matrix. \\
& TGA & Gradient Ascent applied to the unbiased risk estimator with true transition matrix. \\
\hline
DM~\cite{gao2021discriminative} & - & Discriminative Models with Weighted Loss. \\
\hline
FWD~\cite{fwd2018} & - & Forward Correction. \\
\hline
\multirow{3}{4em}{CPE~\cite{cpe2023}} & I & Complementary Probability Estimates. \\
& F & Complementary Probability Estimates with true transition matrix. \\
& T & Complementary Probability Estimates with trainable transition matrix. \\
\hline
\multirow{3}{4em}{MCL~\cite{mcl2020}} & MAE & Multiple Complementary Loss with mean absolute error. \\
& EXP & Multiple Complementary Loss with exponential loss. \\
& LOG & Multiple Complementary Loss with negative log loss. \\
\bottomrule
\end{tabular}%
}}
\end{table}
\section{Broader impacts}
\label{sec:borader-impacts}
The library may advance the algorithms for learning from complementary labels. Those algorithms could learn a classifier with weak information. The privacy of the users may be easier to compromised as a result. We suggest the practitioners pay attention to the privacy issues when trying to utilize the collected datasets and the CLL algorithms.

\section{Access to the dataset and codes for reproduce}
\label{sec:link}
Please refer to the following link: \url{https://github.com/ntucllab/libcll}
